# Supplementary material for: Quantum Machine Learning of Molecular Energies with Hybrid Quantum-Neural Wavefunction
Source: arXiv:2501.04264 source file (2025-09-09)
Supplement: Supplementary file 1 [file si.pdf]

# Supplementary Information for "Quantum Machine Learning of Molecular Energies with Hybrid Quantum-Neural Wavefunction"

Weitang Li,[1,*] Shi-Xin Zhang,[2] Zirui Sheng,[1]
Cunxi Gong,[1] Jianpeng Chen,[1] and Zhigang Shuai[1,3]

[1]*School of Science and Engineering, The Chinese University of Hong Kong, Shenzhen, Guangdong 518172, China*

[2]*Institute of Physics, Chinese Academy of Sciences, Beijing 100190, China*

[3]*Department of Chemistry, MOE Key Laboratory for Organic OptoElectronics and Molecular Engineering, Tsinghua University, Beijing 100084, China*

[*] liwt31@gmail.com

## I. PUNN HYPERPARAMETERS

In Table I we list the hyperparameters of the pUNN model employed in this work. Here $N$ is the number of spatial orbitals.

TABLE I. Hyperparameters of the pUNN Model

| **Hyperparameter** | **Value** |
|---|---|
| | **Quantum Circuit** |
| Circuit depth | Linear in $N$, approximately 20 for $N = 8$ |
| Number of parameters | approximately $N^2/4$ |
| Optimizer (noiseless simulation) | L-BFGS-B |
| Optimizer (quantum hardware) | SOAP |
| | **Neural Network** |
| Number of hidden layers | $N - 3$ |
| Neurons per hidden layer | $2KN$ or $4N$ with $K = 2$ |
| Number of parameters | $16N^3 - 52N^2 - 8N + 1$ |
| Activation function | ReLU |
| Optimizer | AdaMax |
| Initial learning rate | 0.01 |
| Momentum parameters | $\beta_1 = 0.8$, $\beta_2 = 0.99$ |
| Learning rate schedule | Linear decay to 0.001 between steps 8000 and 32000 |

## II. ADDITIONAL BENCHMARKS IN THE STRONGLY CORRELATED REGIME

To further test pUNN's performance in strongly correlated regimes, we conduct additional benchmark studies on the potential energy profiles of $N_2$ and $CH_4$ across a range of bond lengths, from equilibrium to dissociation, as shown in Fig. 1. These results complement our existing $H_8$ benchmarks and demonstrate pUNN's robustness. At equilibrium bond lengths or weak correlation, pUNN achieves near-chemical accuracy for both $N_2$ and $CH_4$. As bond lengths increase toward the dissociation limit and the strong correlation regime, pUNN's error grows controllably

and outperforms UCCSD. This is remarkable given pUNN's shallow circuit depth (approximately 20 vs. approximately 1000 for UCCSD) and lower qubit count ($N$ vs. $2N$).

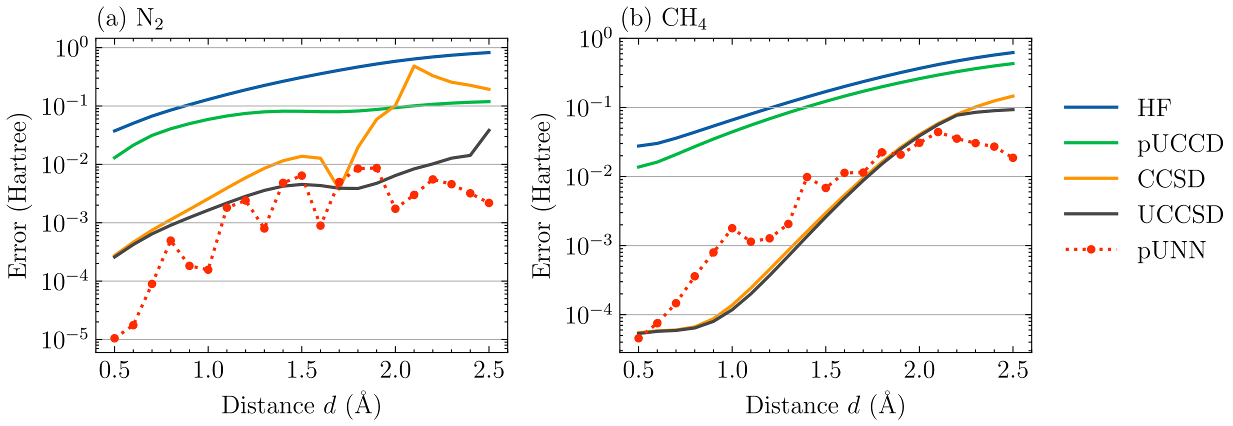


FIG. 1. Benchmarking pUNN based on the potential energy profile of $N_2$ and $CH_4$. (a) The error compared with the exact solution versus the N-N bond length in $N_2$. (b) The error compared with the exact solution versus the C-H bond length in $CH_4$.

## III. THE GEOMETRIES OF THE MOLECULES

$BH_3$

```
B   0.0000   0.0000   0.0000
H   0.0000   1.1900   0.0000
H   1.0306  -0.5950   0.0000
H  -1.0306  -0.5950   0.0000
```

$NH_3$

```
N   0.0000   0.0000   0.0000
H   0.9330   0.0000  -0.3660
H  -0.4665   0.8080  -0.3660
H  -0.4665  -0.8080  -0.3660
```

$CH_4$

```
C   0.0000   0.0000   0.0000
H  -0.6293   0.6293   0.6293
H   0.6293  -0.6293   0.6293
H  -0.6293  -0.6293  -0.6293
H   0.6293   0.6293  -0.6293
```

$NH_4^+$

```
N   0.0000   0.0000   0.0000
H  -0.5889   0.5889   0.5889
H   0.5889  -0.5889   0.5889
H  -0.5889  -0.5889  -0.5889
H   0.5889   0.5889  -0.5889
```

$N_2$

```
N   0.0000   0.0000   0.0000
N   0.0000   0.0000   1.0900
```

CO

```
C  0.0000  0.0000  0.0000
O  0.0000  0.0000  1.1280
```

$C_4H_4$ reactant/product

```
C  0.6750  0.7900  0.0000
H  1.4380  1.5530  0.0000
C -0.6750  0.7900  0.0000
H -1.4380  1.5530  0.0000
C  0.6750 -0.7900  0.0000
H  1.4380 -1.5530  0.0000
C -0.6750 -0.7900  0.0000
H -1.4380 -1.5530  0.0000
```

$C_4H_4$ transition state

```
C  0.7300  0.7300  0.0000
H  1.4930  1.4930  0.0000
C -0.7300  0.7300  0.0000
H -1.4930  1.4930  0.0000
C  0.7300 -0.7300  0.0000
H  1.4930 -1.4930  0.0000
C -0.7300 -0.7300  0.0000
H -1.4930 -1.4930  0.0000
```

We note that the transition state of $C_4H_4$ has an internal instability in RHF calculation and stability check is necessary to ensure convergence to the correct RHF reference state.
